# Supplementary material for: Discretized Halbach spheres: Icosahedral symmetry for optimal field homogeneity
Source: arXiv:2512.17497 source file (2026-03-25)
Supplement: Supplementary file 1 [file Supplementary_Material.pdf]

# SUPPLEMENT to: Towards Halbach Spheres – Icosahedral Symmetry Is Not Just Cool Anymore

Ingo Rehberg\*

*Institute of Physics, University of Bayreuth, 95440 Bayreuth, Germany*

Peter Blümner†

*Institute of Physics, University of Mainz, 55128 Mainz, Germany*

(Dated: December 19, 2025)

## I. LIST OF SYMBOLS USED IN THE ARTICLE

|                                     |                                                                                                                                              |               |
|-------------------------------------|----------------------------------------------------------------------------------------------------------------------------------------------|---------------|
| $a$ :                               | Edge length of a polyhedron,                                                                                                                 | p.3           |
| $\mathbf{B}, B_x, B_y, B_z$ :       | Magnetic induction or $B$ -field, components,                                                                                                | p. 2, Eq.(1)  |
| $B_c$ :                             | Magnitude of the $B$ -field at the center of the polyhedron,                                                                                 | p.2, Eq. (5)  |
| $B_0$ :                             | $\frac{2\mu_0 m}{4\pi(a/2)^3}$ , maximum magnetic field of a dipole at distance $a/2$ , for spheres of radius $a/2$ : $B_0 = \frac{2}{3}B_R$ | p.4, Fig.3    |
| $B_R$ :                             | Remanent magnetic flux density (remanence)                                                                                                   | p.2, Eq.(2)   |
| $d$ :                               | Distance from the center (a positive number)                                                                                                 | p.4, Fig.11   |
| $D_c, D_s$ :                        | edge length of a cubical and diameter of a spherical magnet                                                                                  | Eq.(C4)(C5)   |
| $f_\lambda$ :                       | Flux-like homogeneity parameter                                                                                                              | p.6           |
| $\mathbf{E}(k)$ :                   | Complete elliptic integral, 2. kind, modulus $k$                                                                                             | p.2, Eq.(6)   |
| $h$ :                               | Thickness of a magnetic disk (along the $z$ -axis)                                                                                           | p.2, Eq.(5)   |
| $\mathbf{m}$ :                      | Magnetic dipole moment,                                                                                                                      | p. 13         |
| $m$ :                               | mode number of spherical harmonic                                                                                                            | p.12, Eq.(E2) |
| $\mathbf{M}$ :                      | Magnetization vector                                                                                                                         | p.2, Eq.(2)   |
| $p$ :                               | Position along an axis, including sign                                                                                                       | Fig.3         |
| $\mathbf{r}, \hat{\mathbf{r}}, r$ : | Position vector, unit vector, magnitude                                                                                                      | p.2, Eq.1     |
| $R_{\text{in}}, R_{\text{out}}$ :   | Inner and outer radius of a spherical or cylindrical shell                                                                                   | p.2, Eq.(5)   |
| $r_s$ :                             | Radius of spheres in contact, $a/2$                                                                                                          | p.4           |
| $R$ :                               | Circumradius of a Platonic or Archimedean solid                                                                                              | p.3, Table I  |
| $v_r$ :                             | The ratio of the volume of magnets over that of the corresponding shell                                                                      | p.3, Eq.(8)   |
| $F, V, E$ :                         | Faces, vertices and edges of a polyhedron                                                                                                    | p.3, Table I  |
| $x_i, y_i, z_i$ :                   | Cartesian coordinates of vertices, index $i$                                                                                                 | suppl. II.    |
| $\alpha_o$ :                        | Angle of orientation of magnetization relative to the orientation axis,                                                                      | p.2, Eq.(3)   |
| $\eta$ :                            | Shorthand notation for $r_s/R$                                                                                                               | Eq.(C7)       |

---

\* [Ingo.Rehberg@uni-bayreuth.de](mailto:Ingo.Rehberg@uni-bayreuth.de)

† [bluemler@uni-mainz.de](mailto:bluemler@uni-mainz.de)

|                         |                                                                                                    |                     |
|-------------------------|----------------------------------------------------------------------------------------------------|---------------------|
| $\kappa$ :              | The curvature of $B$ -profiles                                                                     | Eq.(9)              |
| $\theta_{\mathbf{p}}$ : | Angle of position of a dipole,                                                                     | page 2, Eq.(3)      |
| $\theta$ :              | Polar angle of spherical coordinates                                                               | Eq.(A1)             |
| $\phi$ :                | Azimuthal angle, spherical and cylinder coordinates                                                | Eq.(A1)             |
| $\varphi$ :             | Golden ratio $\frac{1+\sqrt{5}}{2}$ , satisfying $\varphi^2 = \varphi + 1$                         | APP. D, Suppl. p.2, |
| $\Phi_{\mathbf{m}}$ :   | Magnetic scalar potential                                                                          | App(E)              |
| $\lambda$ :             | Characteristic decay length, measured in units of $r_s$ ,                                          | Fig.3               |
| $\rho$ :                | Position along the three Cartesian axes                                                            | Fig.3               |
| $\Psi$ :                | Sphericity of polyhedra: Surface-area ratio of a volume-equivalent sphere to the polyhedron itself | SU p.2              |

## II. PROPERTIES OF THE PLATONIC AND TWO RELEVANT ARCHIMEDEAN SOLIDS

In this section, additional geometric characteristics of the five Platonic solids and the two Archimedean solids referenced in the main text are provided. The emphasis is on practical details that facilitate physical construction. You may also consult the Python code below (see III), which generates the corresponding arrangements and can produce STL files via **OpenSCAD** for 3D printing support structures.

If you prefer to generate the solids by another method, the coordinates of the vertices (representing the locations of the magnets) will be particularly useful. They are listed such that the resulting magnet has its field oriented along the  $x$ -axis, consistent with the convention used in the main publication.

The notation of the following list is such that the center of each magnet (vertex of the polyhedron) is located at

$$x_i = R \hat{x}(i) \quad \text{for } i = 1..N,$$

where  $x_i$  denotes the Cartesian  $x$ -coordinate of the  $i^{\text{th}}$  magnet center (and analogously for  $y_i$  and  $z_i$ ): Here,  $N$  is the total number of vertices/magnets, and  $R$  is the distance from the center/origin. The unit vectors ( $\hat{x}(i)$ ,  $\hat{y}(i)$ ,  $\hat{z}(i)$ ) are listed below for each polyhedron. Because the magnets must also be correctly oriented, the following algorithmic procedure is applied. Each magnet is first placed at the origin and rotated by an angle  $\alpha_i$  about the  $z$ -axis, where

$$\alpha_i = 2 \tan^{-1} \left( \frac{\sqrt{\hat{y}(i)^2 + \hat{z}(i)^2}}{\hat{x}(i)} \right).$$

It is then rotated by an angle  $\theta_i$  about the  $x$ -axis, with

$$\theta_i = \tan^{-1} \left( \frac{\hat{z}(i)}{\hat{y}(i)} \right),$$

Finally, it is translated to its final position  $R [\hat{x}(i), \hat{y}(i), \hat{z}(i)]$ .

To keep the coordinate lists concise, polyhedron-specific abbreviations are introduced; these apply only within the definition of each individual polyhedron and are not interchangeable between them. In addition to the vertex coordinates, the edge length  $a$  and the sphericity,  $\Psi$ , of each polyhedron are provided. The *golden ratio*  $\varphi$  is also used frequently.

### A. Tetrahedron

Edge length:  $a = \frac{4}{\sqrt{6}} R$ .

Sphericity:  $\Psi = \sqrt[3]{\frac{\pi}{6\sqrt{3}}} \approx 0.67$ .

Coordinates:

$$\hat{x}(i) = [T, -T, -T, T],$$

$$\hat{y}(i) = [T, -T, T, -T],$$

$$\hat{z}(i) = [T, T, -T, -T] \quad \text{with} \quad T := \frac{1}{\sqrt{3}}.$$

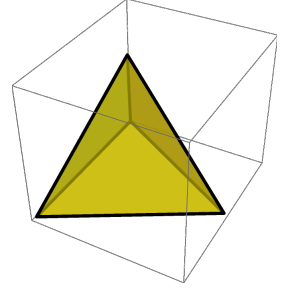

### B. Hexahedron or Cube

Edge length:  $a = \frac{2}{\sqrt{3}} R$ .

Sphericity:  $\Psi = \sqrt[3]{\frac{\pi}{3\sqrt{3}}} \approx 0.85$ .

Coordinates:

$$\hat{x}(i) = [C, -C, C, -C, C, -C, C, -C],$$

$$\hat{y}(i) = [C, C, -C, -C, C, C, -C, -C],$$

$$\hat{z}(i) = [C, C, C, C, -C, -C, -C, -C] \quad \text{with} \quad C := \frac{1}{\sqrt{3}}.$$

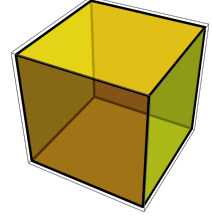

### C. Octahedron

Edge length:  $a = \sqrt{2} R$ .

Sphericity:  $\Psi = \sqrt[3]{\frac{\pi}{6}} \approx 0.81$ .

Coordinates:

$$\hat{x}(i) = [A, -A, A, -A, 0, 0],$$

$$\hat{y}(i) = [A, A, -A, -A, 0, 0],$$

$$\hat{z}(i) = [0, 0, 0, 0, 1, -1] \quad \text{with} \quad A := \frac{1}{\sqrt{2}}.$$

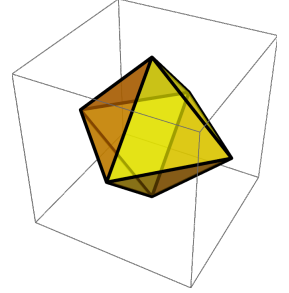

### D. Dodecahedron

Edge length:  $a = \frac{2}{\varphi\sqrt{3}} R$ .

Sphericity:  $\Psi = \frac{\sqrt[3]{180\pi(47+21\sqrt{5})}}{6\sqrt{25+10\sqrt{5}}} \approx 0.91$ .

Coordinates:

$$\hat{x}(i) = [A, -A, A, -A, A, -A, A, -A, 0, 0, 0, 0, B, -B, B, -B, C, -C, C, -C] \quad \text{with} \quad A := \frac{1}{\sqrt{3}},$$

$$\hat{y}(i) = [A, A, -A, -A, A, A, -A, -A, C, -C, C, -C, 0, 0, 0, 0, B, B, -B, -B] \quad \text{with} \quad B := \frac{1}{\varphi\sqrt{3}},$$

$$\hat{z}(i) = [A, A, A, A, -A, -A, -A, -A, B, B, -B, -B, C, C, -C, -C, 0, 0, 0, 0] \quad \text{with} \quad C := \frac{\varphi}{\sqrt{3}}.$$

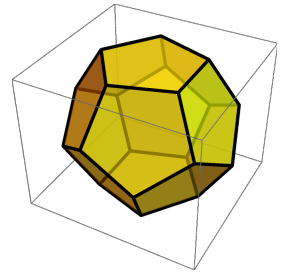

### E. Icosahedron

Edge length:  $a = \frac{2}{\sqrt{\varphi+2}} R$ .

Sphericity:  $\Psi = \sqrt[3]{\frac{(7+3\sqrt{5})\pi}{30\sqrt{3}}} \approx 0.94$ .

Coordinates:

$$\begin{aligned}\hat{x}(i) &= [0, 0, 0, 0, A, -A, A, -A, B, -B, B, -B], \\ \hat{y}(i) &= [A, -A, A, -A, B, B, -B, -B, 0, 0, 0, 0] \quad \text{with } A := \frac{1}{\sqrt{\varphi+2}}, \\ \hat{z}(i) &= [B, B, -B, -B, 0, 0, 0, 0, A, A, -A, -A] \quad \text{with } B := \frac{\varphi}{\sqrt{\varphi+2}}.\end{aligned}$$

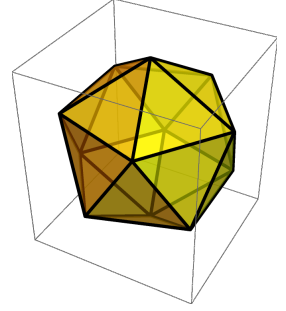

### F. Truncated icosahedron or soccer ball

Edge length:  $a = \frac{4}{\sqrt{58+18\sqrt{5}}} R$ .

Sphericity:  $\Psi = \frac{\sqrt[3]{180\pi(2487+1075\sqrt{5})}}{6(10\sqrt{3}+\sqrt{25+10\sqrt{5}})} \approx 0.97$ .

Coordinates:

$$\begin{aligned}\hat{x}(i) &= [0, 0, 0, 0, A, A, -A, -A, E, E, -E, -E, B, B, B, B, -B, -B, -B, -B, F, F, F, F, -F, -F, -F, -F, \dots \\ &\quad \dots C, C, C, C, -C, -C, -C, -C, A, A, A, A, -A, -A, -A, -A, G, G, G, G, -G, -G, -G, -G, D, D, D, D, -D, -D, -D, -D], \\ \hat{y}(i) &= [A, A, -A, -A, E, -E, E, -E, 0, 0, 0, 0, F, F, -F, -F, F, F, -F, -F, C, C, -C, -C, C, C, -C, -C, \dots \\ &\quad B, B, -B, -B, B, B, -B, -B, G, G, -G, -G, G, G, -G, -G, D, D, -D, -D, D, D, -D, -D, A, A, -A, -A, A, A, -A, -A], \\ \hat{z}(i) &= [E, -E, E, -E, 0, 0, 0, 0, A, -A, A, -A, C, -C, C, -C, C, -C, C, -C, B, -B, B, -B, B, -B, B, \dots \\ &\quad F, -F, F, -F, F, -F, F, -F, D, -D, D, -D, D, -D, D, -D, A, -A, A, -A, A, -A, A, -A, G, -G, G, -G, G, -G, G, -G], \\ \text{with: } A &:= \frac{1}{\sqrt{9\varphi+10}}, \quad B := 2A, \quad C := A\varphi, \quad D := 2C, \\ E &:= 3C, \quad F := (1+2\varphi)A, \quad G := (2+\varphi)A.\end{aligned}$$

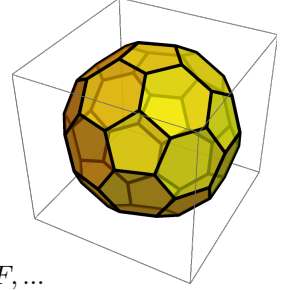

### G. Truncated icosidodecahedron or great rhombicosidodecahedron

Edge length:  $a = \frac{2}{\sqrt{31+12\sqrt{5}}} R$ .

Sphericity:  $\Psi = \frac{\sqrt[3]{900\pi(861+380\sqrt{5})}}{30(1+\sqrt{3}+\sqrt{5+2\sqrt{5}})} \approx 0.97$ .

Coordinates:

$$\begin{aligned}\hat{x}(i) &= [A, A, A, A, -A, -A, -A, -A, M, M, M, M, -M, -M, -M, -M, A, A, A, A, -A, -A, -A, -A, \dots \\ &\quad \dots B, B, B, B, -B, -B, -B, -B, L, L, L, L, -L, -L, -L, -L, C, C, C, C, -C, -C, -C, -C, A, A, A, A, -A, -A, -A, -A, \dots \\ &\quad \dots K, K, K, K, -K, -K, -K, -K, F, F, F, F, -F, -F, -F, -F, E, E, E, E, -E, -E, -E, -E, J, J, J, J, -J, -J, -J, -J, \dots \\ &\quad \dots D, D, D, D, -D, -D, -D, -D, C, C, C, C, -C, -C, -C, -C, H, H, H, H, -H, -H, -H, -H, G, G, G, G, -G, -G, -G, -G], \\ \hat{y}(i) &= [A, A, -A, -A, A, A, -A, -A, A, A, -A, -A, A, A, -A, -A, M, M, -M, -M, M, M, -M, -M, C, C, -C, -C, C, C, -C, -C, \dots \\ &\quad \dots B, B, -B, -B, B, B, -B, -B, L, L, -L, -L, L, L, -L, -L, F, F, -F, -F, F, F, -F, -F, A, A, -A, -A, A, A, -A, -A, \dots \\ &\quad \dots K, K, -K, -K, K, K, -K, -K, D, D, -D, -D, D, D, -D, -D, E, E, -E, -E, E, E, -E, -E, J, J, -J, -J, J, J, -J, -J, \dots \\ &\quad \dots G, G, -G, -G, G, G, -G, -G, C, C, -C, -C, C, C, -C, -C, H, H, -H, -H, H, H, -H, -H], \\ \hat{z}(i) &= [M, -M, M, -M, M, -M, M, -M, A, -A, A, -A, A, -A, A, -A, A, -A, A, -A, L, -L, L, -L, L, -L, L, -L, \dots \\ &\quad \dots C, -C, C, -C, C, -C, C, -C, B, -B, B, -B, B, -B, B, -B, K, -K, K, -K, K, -K, K, -K, F, -F, F, -F, F, -F, F, -F, \dots \\ &\quad \dots A, -A, A, -A, A, -A, A, -A, J, -J, J, -J, J, -J, J, -J, D, -D, D, -D, D, -D, D, -D, E, -E, E, -E, E, -E, E, -E, \dots \\ &\quad \dots H, -H, H, -H, H, -H, H, -H, G, -G, G, -G, G, -G, G, -G, C, -C, C, -C, C, -C, C, -C],\end{aligned}$$

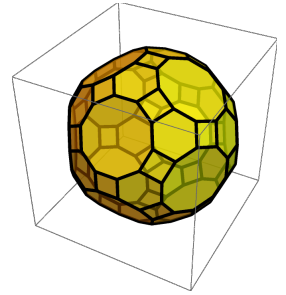

$$\begin{aligned}\text{with: } A &:= \frac{1}{\sqrt{19+24\varphi}}, \quad B := 2A, \quad C := \sqrt{\frac{14+9\varphi}{241}}, \quad D := 2\sqrt{\frac{19-5\varphi}{241}}, \quad E := \frac{\sqrt{5}}{2}D, \quad F := \sqrt{\frac{23+32\varphi}{241}}, \\ G &:= \frac{3}{2}D, \quad H := 2C, \quad J := \sqrt{5}C, \quad K := \sqrt{\frac{175-8\varphi}{241}}, \quad L := \sqrt{\frac{55+87\varphi}{241}}, \quad M := \sqrt{\frac{155+48\varphi}{241}}.\end{aligned}$$

### III. PYTHON SCRIPT FOR CONSTRUCTING THE TRUNCATED ICOSIDODECAHEDRON

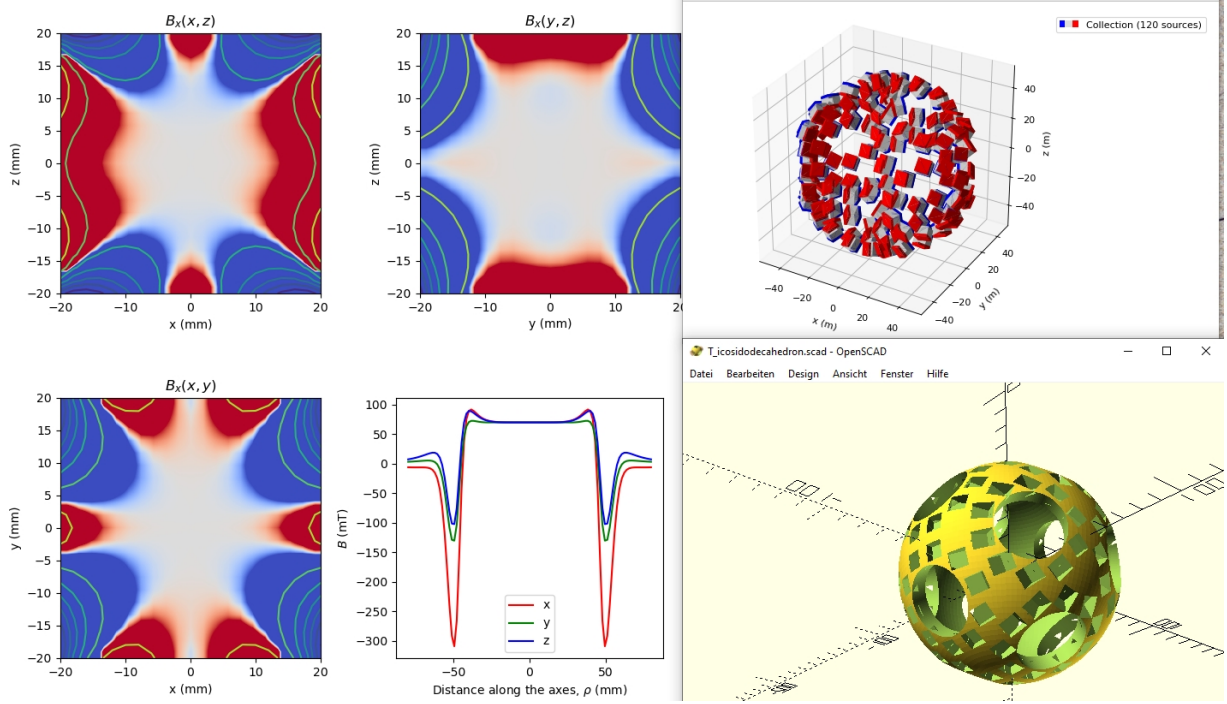

FIG. 1. A screenshot from the production process of the truncated icosidodecahedron with the Python script listed below. The upper right image shows the location of the cubical magnets. The 4 figures to its left give an impression of the central saddle point by showing the field in 3 planes, and a quantitative plot along the 3 axes in the xy-plane. The lower right part shows the scad file produced by this program using OpenSCAD.

The Python script listed below demonstrates the first step in the construction process of a Halbach-sphere discretized by 120 magnets at the vertices of a truncated icosidodecahedron. It employs the `magpylib` library (<https://magpylib.readthedocs.io/en/stable/>) to distribute and align the 120 magnets, and to compute and visualize the magnetic field in the central planes. `SolidPython` (<https://github.com/SolidCode/SolidPython>) is subsequently used to create a corresponding `scad` file for the support of the 120 magnets. That `scad` file can be rendered in `OpenSCAD` (<https://openscad.org/>) and exported as an STL file for 3D printing.

```

1  """Code for Supplemental material, Dec 12 2025.
2
3  Generates a Halbach-sphere approximated by an arrangement of magnets on a
4      TRUNCATED ICOSIDODECAHEDRON
5
6  """
7  try:
8      from solid import cube, cylinder, translate, rotate, scad_render_to_file, sphere
9  except ImportError:
10     from solid2 import cube, cylinder, translate, rotate, scad_render_to_file, sphere
11 import magpylib as magpy
12 import matplotlib.pyplot as plt
13 from numpy import atan2, acos, sqrt, array, pi, linspace, meshgrid, zeros, column_stack
14
15 def vertices():
16     """Give vertex coordinates of Truncated icosidodecahedron.
17     https://en.wikipedia.org/wiki/Truncated_icosidodecahedron
18     code from: https://zenodo.org/records/15387951 (list of Archimed. solids)
19     """
20     def p_e(triple):
21         # even permutations of a triple
22         return [triple[i:]+triple[:i] for i in range(3)]
23     def s(j,i):
24         # switching between + and - in intervals of j
25         return (-1)**(i//j)
26     phi = (1. + sqrt(5.)) / 2 # golden mean
27     verts = [] # list for the 120 vertices

```

```

25 triples = [(1/phi,      1/phi,      3 + phi), # see wikipedia, link above
26             (2/phi,      phi,       1+2*phi),
27             (1/phi,      phi**2,    3*phi-1),
28             (2*phi-1,    2,         2 + phi),
29             ( phi,       3,         2 * phi)]
30 for i in range(8):
31     for a, b, c in triples:
32         verts.extend(p_e([s(1,i)*a, s(2,i)*b, s(4,i)*c]))
33 return (array(verts)/(2*phi-2)/sqrt(31+12*sqrt(5))*2).T # scale to R=1
34
35 def vertices_alternativ():
36     """Vertex positions. Easier code transport to other progr. languages."""
37     a = 1/sqrt(31+12*sqrt(5))
38     b = 2*a
39     c = sqrt((37+9*sqrt(5))/482)
40     d = sqrt(2*(33-5*sqrt(5))/241)
41     e = sqrt(5)/2*d
42     f = sqrt((39+16*sqrt(5))/241)
43     g = 3/2*d
44     h = 2*c
45     j = sqrt(5*(37+9*sqrt(5))/482)
46     k = sqrt((171-4*sqrt(5))/241)
47     l = sqrt((197+87*sqrt(5))/482)
48     m = sqrt((179+24*sqrt(5))/241)
49     xi = array([
50         a, a, a, a,-a,-a,-a,-a, m, m, m, m,-m,-m,-m,-m, a, a, a, a,
51         -a,-a,-a,-a, b, b, b, b,-b,-b,-b,-b, l, l, l, l,-l,-l,-l,-l,
52         c, c, c, c,-c,-c,-c,-c, a, a, a, a,-a,-a,-a,-a, k, k, k, k,
53         -k,-k,-k,-k, f, f, f, f,-f,-f,-f,-f, e, e, e, e,-e,-e,-e,-e,
54         j, j, j, j,-j,-j,-j,-j, d, d, d, d,-d,-d,-d,-d, c, c, c, c,
55         -c,-c,-c,-c, h, h, h, h,-h,-h,-h,-h, g, g, g, g,-g,-g,-g,-g])
56     yi = array([
57         a, a, -a, -a, a, a, -a, -a, a, a, -a, -a, a, a, -a, -a, m, m, -m, -m,
58         m, m, -m, -m, c, c, -c, -c, c, c, -c, -c, b, b, -b, -b, b, b, -b, -b,
59         l, l, -l, -l, l, l, -l, -l, f, f, -f, -f, f, f, -f, -f, a, a, -a, -a,
60         a, a, -a, a, k, k, -k, -k, k, k, -k, k, d, d, -d, -d, d, d, -d, -d,
61         e, e, -e, -e, e, e, -e, -e, j, j, -j, -j, j, j, -j, -j, g, g, -g, -g,
62         g, g, -g, -g, c, c, -c, -c, c, c, -c, -c, h, h, -h, -h, h, h, -h, -h])
63     zi = array([
64         m, -m, m, -m, m, -m, m, -m, a, -a, a, -a, a, -a, a, -a, a, -a,
65         a, -a, a, -a, l, -l, l, -l, l, -l, l, -l, c, -c, c, -c, c, -c, c, -c,
66         b, -b, b, -b, b, -b, b, -b, k, -k, k, -k, k, -k, k, -k, f, -f, f, -f,
67         f, -f, f, -f, a, -a, a, -a, a, -a, a, -a, j, -j, j, -j, j, -j, j, -j,
68         d, -d, d, -d, d, -d, d, -d, e, -e, e, -e, e, -e, e, -e, h, -h, h, -h,
69         h, -h, h, -h, g, -g, g, -g, g, -g, g, -g, c, -c, c, -c, c, -c, c, -c])
70 return xi, yi, zi
71
72
73 def create_collection(rad, b_r=1.345, a=8):
74     """Return a magpylib Collection."""
75     xi, yi, zi = vertices()
76     alpha = 2*atan2(sqrt(yi**2+zi**2), xi) * 180/pi # spherical Halbach
77     theta = atan2(zi, yi) * 180/pi
78     body = []
79     for j, (alp, the) in enumerate(zip(alpha, theta)):
80         a1 = magpy.magnet.Cuboid(polarization=(b_r, 0, 0), dimension=(a, a, a),
81                                 position=(0, 0, 0), style_color='c')
82         a1.rotate_from_angax(angle=alp, axis='z', anchor=(0, 0, 0))
83         a1.rotate_from_angax(angle=the, axis='x', anchor=(0, 0, 0))
84         a1.move((rad*xi[j], rad*yi[j], rad*zi[j]))
85         body.append(a1)
86     magpy.defaults.display.style.magnet.update({"magnetization":
87         {"mode": 'color',"color": {"mode": 'tricolor',
88                                     "north": 'red', "south": 'blue'}}})
89     return magpy.Collection(body), alpha, theta, xi, yi, zi
90
91 def layout():
92     """Size and distribution of the subplots."""
93     fig = plt.figure(r'Fig-supplemental_code', figsize=(12, 9))
94     axs = [None]*5
95     lin, lil = 0.05, 0.4
96     wid, hei = 0.3, 0.3

```

```

97     bas, ba1 = 0.08, 0.5
98     axs[1] = plt.axes([lin, ba1, wid,    hei])
99     axs[2] = plt.axes([li1, ba1, wid,    hei])
100     axs[0] = plt.axes([lin, bas, wid,    hei])
101     axs[3] = plt.axes([li1, bas, wid-.04, hei])
102     axs[4] = plt.axes([0.65, 0.3, 0.4, 0.4], projection='3d')
103     return fig, axs
104
105 def plt_3(ax, coll):
106     """3 lines along the axes."""
107     x, n = linspace(-80, 80, 101), zeros(101)
108     ax.plot(x, coll.getB(array([x, n, n]).T)[: , 0]*1000, 'r-', label='x')
109     ax.plot(x, coll.getB(array([n, x, n]).T)[: , 0]*1000, 'g-', label='y')
110     ax.plot(x, coll.getB(array([n, n, x]).T)[: , 0]*1000, 'b-', label='z')
111     ax.set(xlabel=r'Distance along the axes, $\rho$ (mm)', ylabel=r'$B$ (mT)')
112     ax.legend()
113
114 def plt_field(coll, rad):
115     """5 plots: magnetic field of collection cll in planes x=0, y=0, z=0."""
116     fig, axs = layout()
117     r_0, b_c = 0.4*rad, coll.getB([0, 0, 0])[0]
118     co = [linspace(-r_0, r_0, 21)]*3
119     for i, pl in enumerate([(0, 1, "$B_x(x,y)$", "x (mm)", "y (mm)"), # 3 planes
120                             (0, 2, "$B_x(x,z)$", "x (mm)", "z (mm)"),
121                             (1, 2, "$B_x(y,z)$", "y (mm)", "z (mm)"]):
122         ct1, ct2 = meshgrid(co[pl[0]], co[pl[1]])
123         pts = column_stack([ct1.ravel() if c == pl[0]
124                             else ct2.ravel() if c == pl[1]
125                             else zeros(ct1.size) for c in range(3)])
126         b2d = array([coll.getB(p) for p in pts]).reshape(ct1.shape+(3,))
127         axs[i].imshow(b2d[:, :, 0], extent=[-r_0, r_0, -r_0, r_0], vmin=b_c*0.999,
128                        vmax=b_c*1.001, interpolation="bilinear", cmap="coolwarm")
129         axs[i].contour(ct1, ct2, b2d[:, :, 0])
130         axs[i].set(xlabel=pl[3], ylabel=pl[4], title=pl[2])
131     print(f'central field B_c = {b_c*1000:1.2f} mT')
132     plt_3(axs[3], coll)
133     magpy.show(coll, canvas=axs[4], backend='matplotlib')
134     axs[4].legend().remove()
135     axs[4].view_init(elev=90, azim=0)
136     plt.show()
137     fig.savefig('Fig_supplemental.pdf', bbox_inches='tight')
138
139 def magnets(xi, yi, zi, alpha, theta):
140     """Define the spaces for 120 magnets to be subtracted."""
141     a = 8
142     mag = []
143     for i, (alp, the) in enumerate(zip(alpha, theta)):
144         c = cube((a, a, a), center=True)
145         c += translate((a/2, 0, 0))(cube((a/10, a, a/10), center=True))
146         c += translate((-a/2, 0, 0))(cube((a/8, a/8, a/8), center=True))
147         c = rotate((0, 0, alp))(c)
148         c = rotate((the, 0, 0))(c)
149         c = translate((xi[i], yi[i], zi[i]))(c)
150         mag = mag + c
151     return mag
152
153 def openings(r_out):
154     """Define the openings for the 6 measurement paths connecting decagons."""
155     hole = 16
156     bo = acos(-sqrt((5+sqrt(5))/10)) * 180/pi
157     h = 3*r_out
158     opn = (cylinder(r=1, h=h, center=True)
159            + rotate((0, bo, 0))(cylinder(r=hole, h=h, center=True))
160            + rotate((0, -bo, 0))(cylinder(r=hole, h=h, center=True))
161            + rotate((90-bo, 0, 0))(cylinder(r=hole, h=h, center=True))
162            + rotate((-90+bo, 0, 0))(cylinder(r=hole, h=h, center=True))
163            + rotate((90, 0, 90-bo))(cylinder(r=hole, h=h, center=True))
164            + rotate((90, 0, -90+bo))(cylinder(r=hole, h=h, center=True)))
165     return opn
166
167 def create_scad(x, y, z, a, t):
168     """SolidPython creates Scad file: sph_out -sph_in -magnets -openings."""

```

```

169     ri, ra = 43, 51 # inner and outer radius (mm) of supporting rings
170     obj = sphere(ra) - magnets(x, y, z, a, t) - sphere(ri) - openings(ra)
171     segments = 128
172     file_out = 'T_icosidodecahedron.scad'
173     scad_render_to_file(obj, file_out, file_header=f'$fn = {segments};')
174     print('>>> wrote Scad-file', file_out)
175
176 if __name__ == '__main__': # create the figure
177     R = 50 # Radius in mm
178     T_Icosi, alpha_m, theta_m, x_m, y_m, z_m = create_collection(R)
179     magpy.show(T_Icosi) # a larger interactive window
180     plt_field(T_Icosi, R) # 5 plots of the field
181     create_scad(R*x_m, R*y_m, R*z_m, alpha_m, theta_m) # make scad file

```
